# Supplementary material for: Understanding the Security Risks of Decentralized Exchanges by Uncovering Unfair Trades in the Wild
Source: arXiv:2401.11547 source file (2024-01-21)
Supplement: Supplementary file 1 [file appendix_journal.tex]

\section{Characterizing Crimes}
\label{sec:behavior}

We further expand the scope of each attack instance by tracing the money flow and smart contract lineage. The goal is to uncover the attack business.

\begin{figure}[!htbp]
\begin{center}
\includegraphics[width=0.495\textwidth]{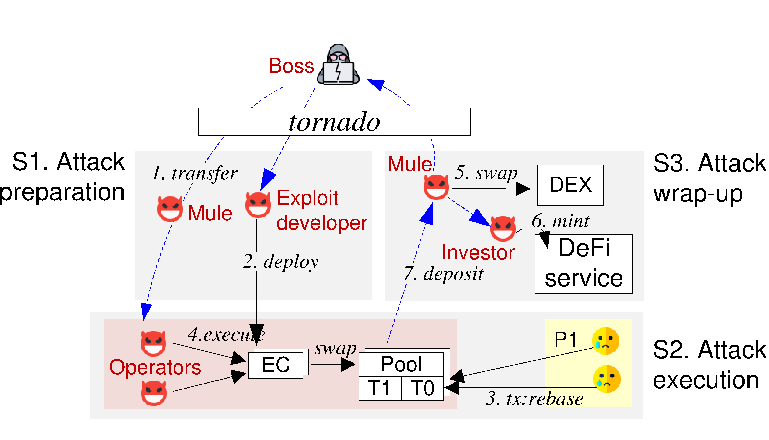}
\end{center}
\caption{Attack campaign template: Preparing, mounting, and wrapping up thefts.}
\label{fig:business}
\end{figure}

Given an attack instance with attacker accounts $\{A\}$, we construct an expanded attack graph by adding the following information: 1) the transactions that pay Ether or tokens to the attacker accounts, 2) the transactions that deploy the smart contracts used in the attack, and 3) the transactions that are sent by the mule accounts which receive the stolen tokens after the attack. These new transactions would add to the graph a set of new accounts, be it either the transaction sender or receiver. We iteratively apply this graph-expansion process until it reaches the ``hub-node'' accounts, which receive or send a large number of transactions (e.g., a popular DEX pool or mixer service). 
For instance, Figure~\ref{fig:business} shows an example of an expanded attack instance, with the attackers in the red box and the victims; the added accounts and transactions are outside the two boxes. 

\noindent
{\bf Attack ecosystem template}: We analyze the expanded attack graph in a template consisting of three phases: 1) attack preparation, 2) attack execution, and 3) attack wrap-up. Phase 2) is the core attack component, and Phases 1) and 3) are the expanded parts. In general, the actual boss often sits behind an exchange/mixer service, such as Tornado~\cite{me:tornado}, to hide its identity. In attack preparation (Phase 1), the boss sends commission in Ether to Attackers and Exploit developers. The Ether transfer can be relayed through the Mules. An Exploit developer writes an Exploit smart contract and deploys it to the blockchain. It then mounts the attack in the execution phase (Phase 2), exercising the strategies described previously (\S~\ref{sec:attack}). To wrap up a series of attacks (Phase 3), the mule receiving the stolen tokens transfers the tokens back to the boss. This is often done by swapping the stolen tokens to ETH (e.g., via DEX and wrapped tokens such as WETH) and by sending the ETH to the boss via a mixer service. In the attack wrap-up phase, the mule may transfer tokens to Investors to maximize the stolen value. 

\begin{table*}[h]
\caption{Attack ecosystem and attacker correlation: Red text shows the two attackers share the same developer of exploit smart contracts. AO represents the attack operator and EC is the exploit smart contract.
}
\label{tab:eco}
\centering{\small
    %\begin{tabular}{|p{0.3cm}|p{0.3cm}|p{0.3cm}|p{1cm}|p{1.2cm}|}
    \begin{tabular}{|c|c|c|c|c|c|c|c|c|}
    \hline
    Accounts & \multicolumn{4}{c|}{Attack (S2)} & \multicolumn{2}{c|}{Preparation (S1)} & \multicolumn{2}{c|}{Wrap-up (S3)}  \\ \cline{2-9}
    (Mules) & \#AO & \#EC & Developer & Value ($10^3$ USD) & Commission & Mixer & DEX & Mixer \\
    \hline
     $0x9799$ & 5 %$0x4e53$, $0xac72$, $0xa084$, $0x5bb4$, $0xe929$ 
& 24 % $0x338c$, $0x3ac7$, $0x34a2$, $0x9a99$, $0x2927$, $0x536b$, $0xe9f8$, $0x684b$, $0x58a3$, $0x72bb$, $0xa8a2$, $0x72cb$, $0x2528$, $0xbf2d$, $0xadfc$, $0xd6a2$, $0x24af$, $0x1335$, $0xf367$, $0x94fc$, $0x5caf$,  $0x6332$, $0x3c3a$, $0x1233$	
& {\bf \color{red} $0x8641$} & 556 & \xmark  & \xmark  & \cmark  & \xmark \\
    \hline
    $0x2a2e$  & 1 %$0x2a2e$ 
& 1 %$0x5f5a$ 
& $0x2a2e$ & 239 & \cmark  & \xmark  & \cmark  & \cmark 
\\
    \hline
    $0xdb40$  & 5 %$0x64bc$, $0x62ae$, $0x3807$, $0x225c$, $0xdb40$ 
& 2 %$0x4dbc$, $0x4626$ 
& $0x4626$ & 113 & \cmark  & \cmark  & \cmark  & \cmark 
\\
    \hline
    $0x0c08$  & 1 %$0xfdee$ 
& 1 %$0x0c08$ 
& $0x0c08$ & 101 & \xmark  & \xmark  & \cmark  & \xmark 
\\
    \hline
    $0x5617$  & 4 %$0x3a51$, $0xf97b$, $0xbf3f$, $0xa1e6$ 
& 10 %$0xfb51$, $0x328d$, $0x8a14$, $0x0fc7$, $0x4ed5$, $0xb439$ ,$0x55a2$, $0x6ba3$ 
& \color{red}{$0x8641$} & 101 & \xmark  & \xmark  & \cmark  & \cmark 
\\
    \hline
    $0xb6bf$ & 1 %$0x675f$ 
& 2 %$0xb6bf$, $0x8526$ 
& $0x675f$ & 20 & \cmark  & \xmark  & \cmark  & \xmark 
\\
    \hline
    $0xc762$ & 1%$0xd0d0$ 
& 1%$0xc762$ 
& $0xd0d0$ & 16 & \cmark  & \cmark  & \cmark  & \cmark 
 \\
    \hline
    $0xa32d$ & 1%$0x7505$ 
& 1%$0xa32d$ 
& $0x7505$ & 6 & \cmark  & \xmark  & \xmark  & \xmark 
\\
    \hline  
    \end{tabular}%
}
\end{table*}

\ignore{
\begin{table}[h]
\caption{Attack ecosystem and attacker correlation: Red text shows the two attack instances are mounted using the exploit smart contracts developed by the same developer. AO represents attack operator and EC is exploit smart contract.
}
\label{tab:eco}
{\centering \scriptsize
    \begin{tabular}{|p{0.3cm}|p{1cm}|p{0.3cm}|p{0.3cm}|p{1cm}|p{0.7cm}|p{0.8cm}|p{.5cm}|}
    \hline
    Idx &Value ($10^3$~USD) & \#AO & \#EC & Developers & Mules & Deposits & Block gaps\\
    \hline
    1 & 552 & 5 %$0x4e53$, $0xac72$, $0xa084$, $0x5bb4$, $0xe929$ 
& 24 % $0x338c$, $0x3ac7$, $0x34a2$, $0x9a99$, $0x2927$, $0x536b$, $0xe9f8$, $0x684b$, $0x58a3$, $0x72bb$, $0xa8a2$, $0x72cb$, $0x2528$, $0xbf2d$, $0xadfc$, $0xd6a2$, $0x24af$, $0x1335$, $0xf367$, $0x94fc$, $0x5caf$,  $0x6332$, $0x3c3a$, $0x1233$	
& {\bf \color{red} $0x8641$} & $0x9799$ & $P_1$ & 121\\
    \hline
    2 & 101 & 1 %$0x2a2e$ 
& 1 %$0x5f5a$ 
& $0x2a2e$ & $0x2a2e$ 
& $P_1$ & 1\\
    \hline
    3 & 96 & 5 %$0x64bc$, $0x62ae$, $0x3807$, $0x225c$, $0xdb40$ 
& 2 %$0x4dbc$, $0x4626$ 
& $0x4626$ & $0xdb40$ 
& $P_1$ & 0\\
    \hline
    4 & 86 & 1 %$0xfdee$ 
& 1 %$0x0c08$ 
& $0x0c08$ & $0x0c08$ 
& $P_1$ & 1\\
    \hline
    5 & 67 & 4 %$0x3a51$, $0xf97b$, $0xbf3f$, $0xa1e6$ 
& 10 %$0xfb51$, $0x328d$, $0x8a14$, $0x0fc7$, $0x4ed5$, $0xb439$ ,$0x55a2$, $0x6ba3$ 
& \color{red}{$0x8641$} & $0x5617$ 
& $P_3$ & 2\\
    \hline
    6 & 48 & 1 %$0x675f$ 
& 2 %$0xb6bf$, $0x8526$ 
& $0x675f$ & $0x675f$ & $P_1$ & 0\\
    \hline
    7 & 29 & 1%$0xd0d0$ 
& 1%$0xc762$ 
& $0xd0d0$ & $0xd0d0$& $P_3$ & 1 \\
    \hline
    8 & 22 & 1%$0x7505$ 
& 1%$0xa32d$ 
& $0x7505$ & $0x7505$& $P_1$ & 0 \\
    \hline  
    \end{tabular}%
}
\end{table}
}

\noindent
{\bf Results}: We measure the attack behavior in terms of attack preparation, execution and wrap-up. We find different attacks mounted by the same mule account are consistent and thus present the aggregated results by mule accounts. The result is in Table~\ref{tab:eco}.

In the attack execution phase (S2), the result shows that attacks are systematic, typically with a mule associated with multiple attack operators (AO) and exploit smart contracts (EC). For instance, Mule $0x9799$ has mounted attacks through $5$ different operator EOAs and leveraged more than $24$ different exploit smart contracts. Her exploit contracts are developed by the same developer for another Mule $0x5617$ (in red in Table~\ref{tab:eco}); this implies an underground business of exploit contract development.

We further characterize the attack preparation (S1) and wrap-up (S3) on different mules. Under S1, Column ``Commission'' shows whether the mule's attack operators receive money used for mounting the attacks within 30 days before the attack. Column ``Mixer'' shows whether the attack commission comes from the anonymized crime boss hidden behind a mixer service, such as Tornado. Under S2, Column ``DEX'' shows whether the attacker interacts with a DEX service to exchange tokens or to maximize the illicit profit. Column ``Tornado'' shows whether the attacker eventually transfer money to the anonymized boss behind the mixer service. The result shows that different mules vary in their strategies in attack preparation and wrap-up. For instance, Mule $0x9799$ is quite simplistic in the sense that she only interacted with DEX and did not involve any mixer service in her attacks. Mule $0xdb40$\footnote{The full address of $0xdb40$ is $0xdb40ea5b6d0ef9e45c00c194345b44765a53dd19$ and the account behavior is public on \url{https://etherscan.io/address/0xdb40ea5b6d0ef9e45c00c194345b44765a53dd19}.} and $0xc762$, on the other hand, are quite sophisticated and employ strategies involving mixer and DEX.

\section{Measuring Liquidity Migration to Uniswap V3}

In deployment, we view Uniswap-V2 and V3 as two co-existing DEX instances, instead of one to replace the other. Because it is costly for liquidity providers to migrate their value from one DEX to another, as analyzed and measured below.

%\subsection{Measuring Liquidity Migration to Uniswap V3}

\begin{figure}[!ht]
  \begin{center} 
    \subfloat[Number of migration transactions over all Uniswap-V2 pools]{%
       \includegraphics[width=0.24\textwidth]{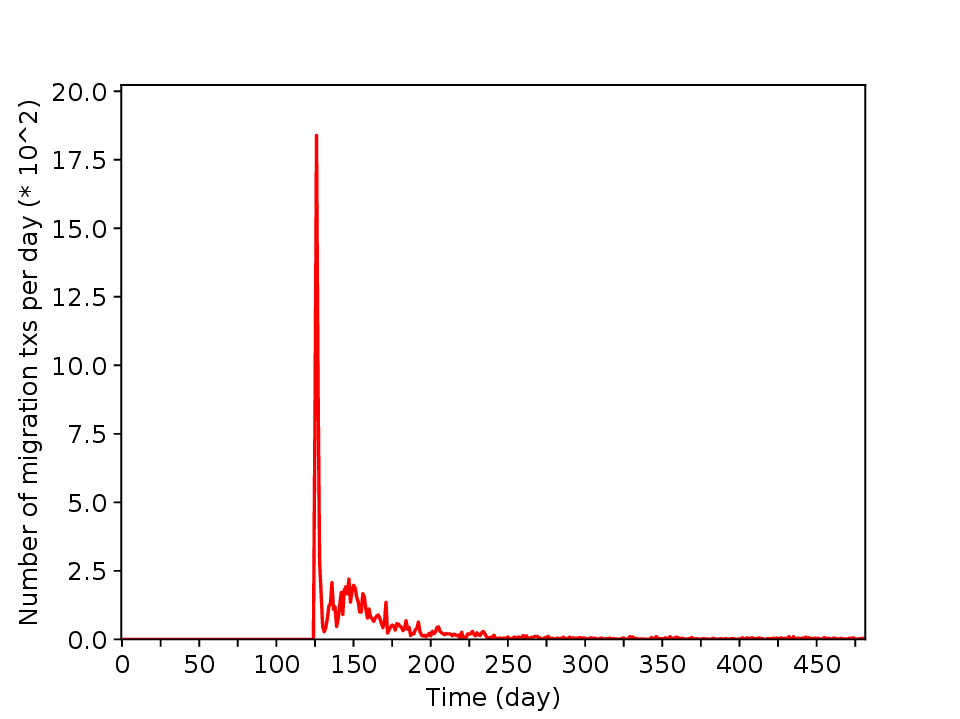} 
       \label{fig:migrate1}
    }%
    \subfloat[The percentage of migrated tokens on top-three Uniswap-V2 pools]{%
       \includegraphics[width=0.24\textwidth]{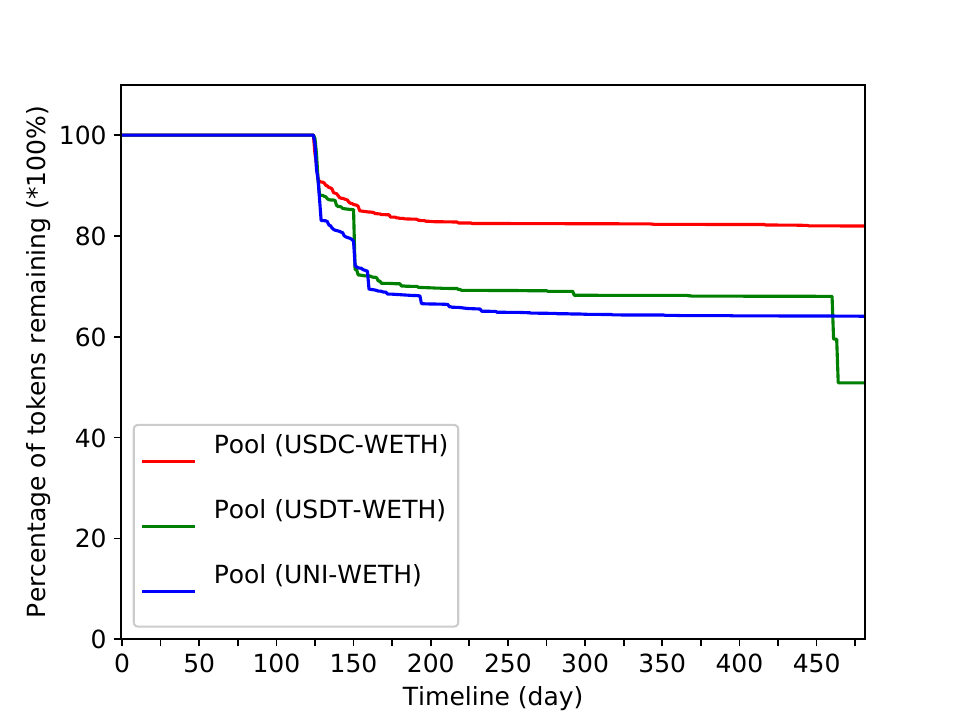} 
       \label{fig:migrate3}
    }%
 \caption{Token/value migration out of Uniswap-V2}
  \end{center}
\end{figure}

The success of a patched pool relies on how much the new pool can attract enough liquidity from existing and new providers. It would be relatively easy for a new liquidity provider to use the patched smart contract. However, it would pose a challenge for existing ``small-business'' liquidity providers to migrate their investment from Uniswap-V2 to Uniswap-V3. The obstacle comes from the relatively high transaction fees compared to the small-volume assets owned by the non-professional, retail providers.

%Another direction to mitigate attacks is to develop patched smart contracts for an AMM pool and deploy them to new blockchain addresses. This approach entails migrating {\it both} liquidity providers and traders to the new pool smart contracts. Note that migrating only traders is insufficient, as the new pool without liquidity providers means a pool without sufficient reserves, which are less attractive to traders. However, in DEX, each liquidity provider is typically an average token owner who invests a small amount in the pool reserves (i.e., a non-professional, retail investor). Such retail provider making small investments would be deterred by the high transaction fees to migrate their invested tokens to a new pool smart contract.

In practice, the difficulty of migrating existing liquidity providers is real. We conducted a measurement study on the Uniswap-V2 using the method as follows: Given that Uniswap deployed a smart contract facilitating migration\footnote{Address of this smart contract is \url{https://etherscan.io/address/0xa5644e29708357803b5a882d272c41cc0df92b34\#code}.}, we collected all the transactions received by this smart contract, joined transaction hashes against the contract's event log, and extracted the contract-call arguments representing the migrated tokens and value. Figure~\ref{fig:migrate1} plots the number of migration transactions per day over time in a $481$-day period. The number of migration transactions spikes at $1839$ transactions on Day $125$ when Uniswap-V3 was launched, then quickly drop, and eventually remains below $9$ transactions per day after Day $250$.
Figure~\ref{fig:migrate3} plots the percentage of tokens remaining in the pool over time. Before Day $125$ when Uniswap-V3 is launched, all three pools have $100\%$ tokens. For all three pools, most drops of token reserves occur within $80$ days after the launch of Uniswap-V3, after which the remaining tokens in a pool become stabilized. The only exception is a dip that occurs around Day $480$ on Pool $USDT-WETH$. Eventually, the remaining tokens in the three pools ($USDC/UNI/USDT$) converge at $80\%/62\%/50\%$.
At last, the difficulty and high cost of migrating providers out of Uniswap-V2 are corroborated by online user complaints~\cite{me:migratev3:complaint1,me:migratev3:complaint2}.
