# Supplementary material for: Understanding the Security Risks of Decentralized Exchanges by Uncovering Unfair Trades in the Wild
Source: arXiv:2401.11547 source file (2024-01-21)
Supplement: Supplementary file 2 [file appendix_yibo.tex]

\ignore{
\section{Measuring Extractable Value}

We take a snapshot of the reserve state stored in Uniswap-V2 pool contract and the balance of the pool stored in token contract on Jan 29, 2022. We get a pair of tokens' reserve states by calling $getReserve()$ to $46170$ Uniswap-V2 pool contract. We get the actual balance of the token that is owned by the pool by calling $balanceOf()$ to each token contract. We find that in $1182$ Uniswap-V2 pool, the reserve in pool contract and the balance in token contract are not the same which means they are not syncing correctly. By leveraging this difference, an attacker can make a benefit of a total $78188.00$ USD from this $1182$ unsynchronized pool. We list the top 10 pools with the most extractable value in Table~\ref{tab:top10valuepool}.
\begin{table}[!htbp] %force in current page, disable float.
  \caption{Top 10 extractable value pool}
  \label{tab:top10valuepool}\centering{\small
  \begin{tabularx}{0.475\textwidth}{ |X|c| } %X is stretching to \textwidth, while c is to match with text width in cell.
    \hline
  Pool & Value extractable (USD) \\ \hline
  FFF - WETH & $4.53*10^4$  \\ \hline
  DEFI5 - WETH & $3.21*10^4$  \\ \hline
  XBE - EURxb & $476.69$  \\ \hline
  PROPHET - ROOT & $36.55$  \\ \hline
  WETH - ENCORE & $26.25$  \\ \hline
  WETH - R34P & $26.13$  \\ \hline
  CommonWealth Credit V1 - DAI  - aDAI & $19.71$  \\ \hline
  vMOON - WETH & $13.12$  \\ \hline
  DEFLCT - BLISS & $11.51$  \\ \hline
  USDN - HULK & $9.82$  \\ \hline
\end{tabularx}
}
\end{table}
}

\ignore{
\clearpage
\section{Discussion: The Case of Uniswap V3}

\subsection{Protocol and API}

\begin{table}[!htbp] %force in current page, disable float.
\caption{Uniswap V3's liquidity pools' API to support token swaps}
\label{tab:uniswapv3:api}\centering{\small
\begin{tabularx}{0.475\textwidth}{ |c|X| } %X is stretching to \textwidth, while c is to match with text width in cell.
  \hline
Version & Function signature \\ \hline
\multirow{2}{*}{V3} & pool.swap(to\_address, amountIn, Price, tokenIn, tokenOut, fee) \\ \cline{2-2}
& uniswapV3SwapCallback(amountIn, amountOut, tokenIn, tokenOut, fee) require(msg.sender == pool)
\\ \hline
\end{tabularx}
}
\end{table}

\begin{table*}[!htbp] %force in current page, disable float.
\caption{Risky swaps on Uniswap V3}
\label{tab:1}\centering{\footnotesize
\begin{tabularx}{0.8\textwidth}{ |X|c|c|c|X| } %X is stretching to \textwidth, while c is to match with text width in cell.
  \hline
  Swap types                & \# of \texttt{deposit} & \# of  \texttt{withdrawal} & Value/diff (\$M) & Causes \\ \hline
  \multicolumn{5}{|l|}{Uniswap V2}   \\  \hline
 Type-I  & $1.9*10^6$  & $1.9*10^6$   & $7.3*10^8$  & Atomic \\ \hline
 Type-III (O) & $4$ & $4$ & $840$ & \textcolor{red}{Router error} \\ \hline
 Type-III (U) & $32$ & $0$ & {\bf $4*10^3$} &  \\  \hline

\end{tabularx}
}
\end{table*}
}
