# Supplementary material for: Understanding the Security Risks of Decentralized Exchanges by Uncovering Unfair Trades in the Wild
Source: arXiv:2401.11547 source file (2024-01-21)
Supplement: Supplementary file 4 [file appendix_outdated.tex]

\section{Usage of Uniswap V3}
\label{sec:v3:use}

\begin{figure}[!ht]
\begin{center}
\includegraphics[width=0.5\textwidth]{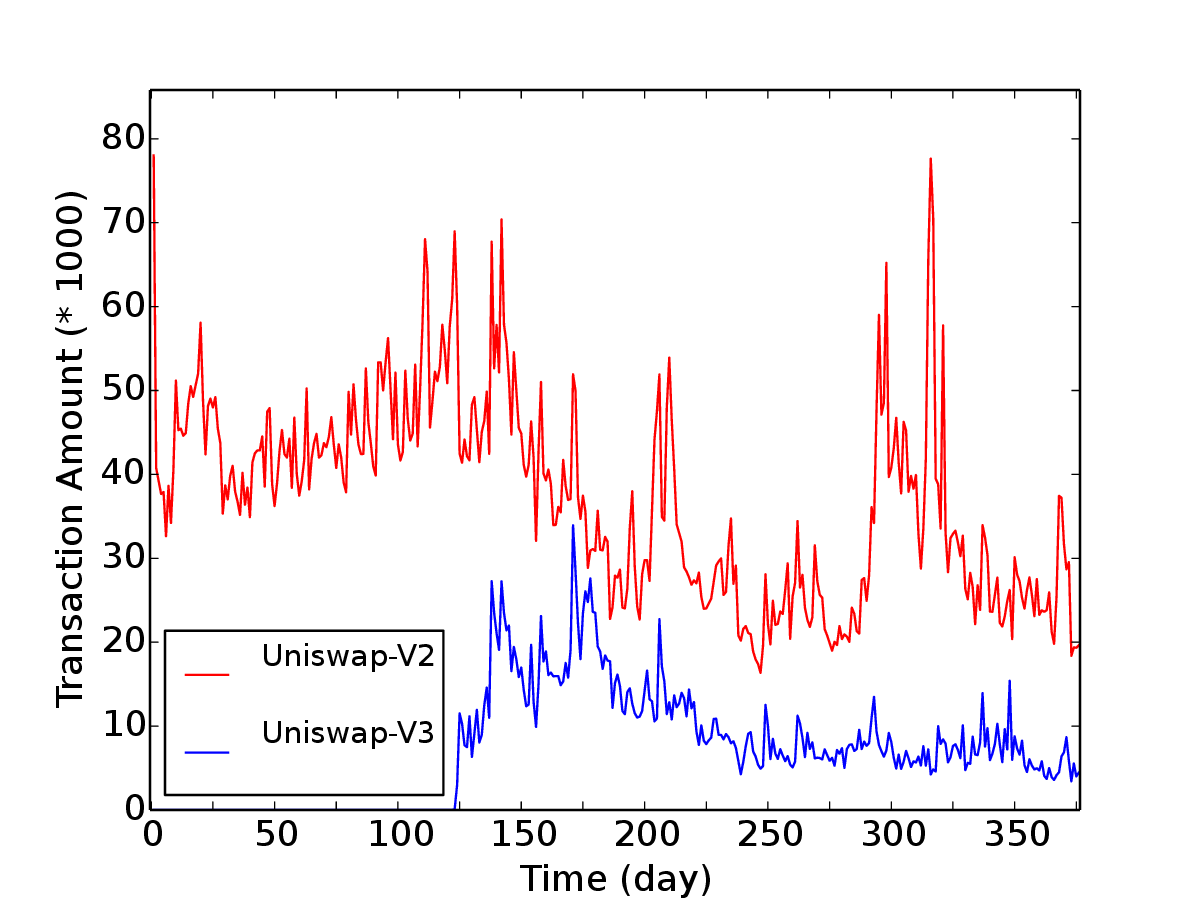}
\end{center}
\caption{Usage of Uniswap V2 and V3 over time}
\label{fig:use}
\end{figure}

We count the transaction amount that interacts with the top $10$ Uniswap pools each day from Jan 1, 2021 to Jan 12, 2022 in both V2 and V3. 
In Figure~\ref{fig:use}, we can see no transaction interacts with Uniswap-V3 in around the first $120$ days because Uniswap-V3 was released on May 5, 2021. After Uniswap-V3 was released, the transaction amount of Uniswap-V2 has no significant decline. On day $371$, the transaction amount of V2 is more than $3$ times than V3. This result shows that Uniswap-V2 has a much larger usebase than Uniswap-V3, months after V3's launch.
